# Supplementary material for: A Nonminimal Coupling Model and its Short-Range Solar System Impact
Source: arXiv:1407.2751 source file (2014-07-10)
Supplement: Supplementary file 1 [file appendixA.tex]

\chapter{Long range curvature solution for $r<R_S$}
\label{ap:curvature}

Here it is computed the curvature solution inside a spherical body, $r<R_S$, so that the curvature equation \eqref{U-equation-simplified} becomes 
\begin{equation}\label{U-equation-simplified-inside}
\frac{d }{ dr}\left(U - 2 f^2_{R0} \rho^{\rm s} \right) = \frac{\eta(t) }{ 4\pi} \frac{M(r) }{ r^2},
\end{equation}
with $M(r)$ as the gravitational mass inside a sphere of radius $r$, defined by
\begin{equation}
M(r) \equiv 4\pi \int_0^r \rho^{\rm s}(\xi) \xi^2 d\xi~~,~~M_{\rm S} = M(R_S).
\end{equation}
As the potential $U$ must be continuous, it helps the calculations to change to a dimensionless variable defined as $x \equiv r/R_S$ and to a dimensionless function $y(x)$ written as
\begin{equation}\label{y-definition}
y\equiv \frac{U(x)}{U(x=1)} = -\frac{4\pi R_S U(x)}{\eta(t)M_{\rm S} }.
\end{equation}
Hence, the curvature equation inside the body (\ref{U-equation-simplified-inside}) becomes
\begin{equation}\label{U-equation-simplified-inside-dim}
\frac{d }{ dx}\left( y + \frac{8\pi f^2_{R0} }{\eta(t) }\frac{R_S}{M_{\rm S}} \rho^{\rm s} \right) = -\frac{M(x) }{ M_{\rm S} x^2 }.
\end{equation}
To compute $y(x)$ from this equation it is necessary to know the density profile inside the spherical body, $\rho^{\rm s}$, so it is assumed that the latter may be expanded as a Taylor series,
\begin{equation}
\label{rhoTaylor} \rho^{\rm s } = \rho^{\rm s}_0 \sum_{i=0} a_i x^i ,
\end{equation}
where $\rho^{\rm s}_0 \sim 10^5~{\rm kg/m^3}$ is the central density and $a_0 = 1$. Therefore
\begin{equation} M (r) = 4\pi \rho^{\rm s}_0 R_S^3 \sum_{i=0} \frac{a_i}{i+3}x^{i+3} ,
\end{equation}
so that
\begin{equation}\label{total-mass}
M_{\rm S} = 4\pi \rho^{\rm s}_0 R_S^3 \sum_{i=0} \frac{a_i}{i+3} .
\end{equation}
Thus, Eq. (\ref{U-equation-simplified-inside-dim}) may be integrated between $x$ and $x=1$ to obtain
\begin{equation}\label{U-equation-simplified-inside-dim-solution}
y = \frac{ \sum_{i=0} \frac{a_i}{i+2} }{ \sum_{i=0} \frac{a_i}{i+3} } - \frac{\sum_{i=0} a_i x^i \left[ \frac{2 f^2_{R0} }{\eta(t) R_S^2} + \frac{x^2}{(i+2)(i+3)} \right] }{ \sum_{i=0} \frac{a_i}{i+3}},
\end{equation}
which with Eq. (\ref{eq:potentialdef}), allows to obtain
\begin{equation}\label{perturbativecondition}
\frac{R_1}{R_0} = \frac{\eta }{ 4\pi [ 2 f^2_{RR0} (\rho^{\rm cos} + \rho^{\rm s}) - f^1_{RR0} ]} \frac{M_{\rm S} }{R_0 R_S}y.
\end{equation}
A thorough discussion on this result may be found in Ref. \cite{solar}.
